# Supplementary material for: A new generation of effective core potentials from correlated calculations: 4s and 4p main group elements and first row additions
Source: arXiv:1907.08658 ancillary file (2019-10-09)
Supplement: Supplementary file 1 [file Supplementary.pdf]

# Supplementary Material: A new generation of effective core potentials from correlated calculations: 4s and 4p main main group elements and first row additions

Guangming Wang[1,†*] and Abdulgani Annaberdiyev[1,†], Cody A. Melton[1,2], M. Chandler Bennett[3], Luke Shulenburger[2], and Lubos Mitas[1]
*1) Department of Physics, North Carolina State University, Raleigh, North Carolina 27695-8202, USA*

*2) Sandia National Laboratories, Albuquerque, New Mexico 87123, USA*
*and*
*3) Oak Ridge National Laboratories, Oak Ridge, Tennessee, 37831, USA[†]*
(Dated: October 9, 2019)

## I. FINITE BASIS ERROR

Figure 1 shows the molecular binding energy discrepancies of SeO for various core approximations compared to AE CCSD(T) calculation in 5Z and CBS limit. The difference of 5Z compared to extrapolated graph is marginal because of the proper cancellation of basis error. Therefore, we conclude that 5Z basis discrepancies are accurate enough to show the quality of ECPs as mentioned in the paper.

We provide selected data to show the completeness or accuracy of the AE basis sets in describing ccECP orbitals. Table I shows an example of this for Ga atom where we carried out ROHF calculations of many atomic states using AE uncontracted aug-cc-pwCVXZ basis sets (X = T, Q, 5). The extrapolated results (CBS) are then compared to numerical results which are free from basis set error. We can see that individual energies and gap differences for various states agree within 0.01 eV.

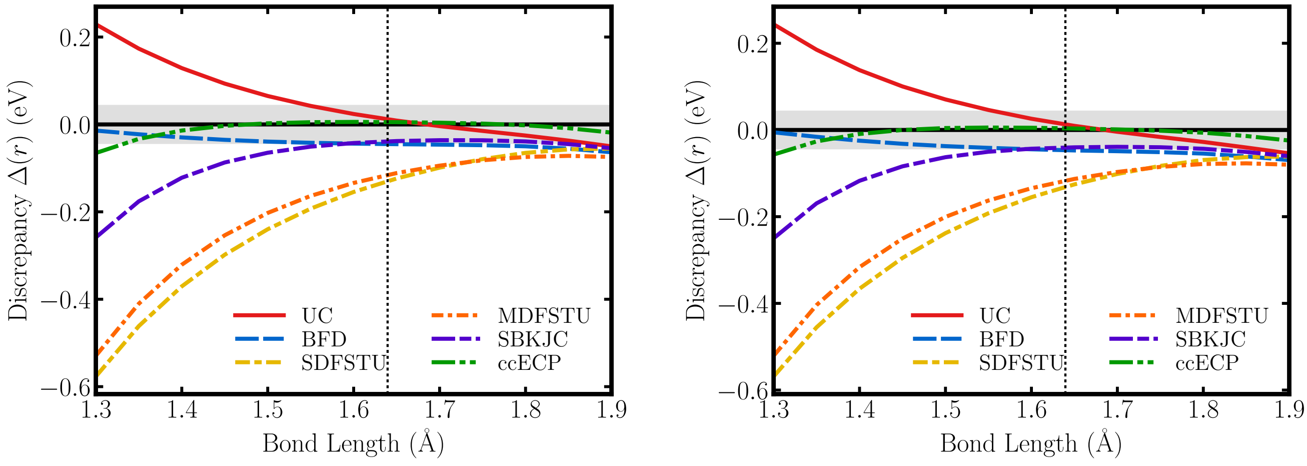


(a) SeO 5Z binding curve discrepancies

(b) SeO extrapolated binding curve discrepancies

FIG. 1: Binding energy discrepancies for (a) SeO 5Z and (b) SeO extrapolated molecules. The binding curves are relative to the CCSD(T) binding curve. The shaded region indicates a discrepancy of chemical accuracy in either direction.

*Electronic address: gwang18@ncsu.edu
†These authors contributed equally to this work

TABLE I: ROHF calculations of Gallium ccECP using AE uncontracted aug-cc-pwCVXZ basis sets (X = T, Q, 5) compared to numerical results (Num.). All data is in Hartree (Ha), except for the last column "Gap Diff." which is in eV.

| SCF | | TZ | QZ | 5Z | CBS | Num. | CBS Gaps | Num. Gaps | Gap Diff. (eV) |
|---|---|---|---|---|---|---|---|---|---|
| [Ar] $3d^{10}4s^24p^1$ | $^2P$ | -1.983806 | -1.984111 | -1.984113 | -1.984120 | -1.984122 | 0.000000 | 0.000000 | 0.000000 |
| [Ar] $3d^{10}4s^24p^2$ | $^2P$ | -1.981656 | -1.982412 | -1.982416 | -1.982435 | -1.982451 | 0.001685 | 0.001671 | 0.000391 |
| [Ar] $3d^{10}4s^14p^2$ | $^4P$ | -1.864691 | -1.865635 | -1.865647 | -1.865665 | -1.865685 | 0.118455 | 0.118437 | 0.000491 |
| [Ar] $3d^{10}4s^24d^1$ | $^2D$ | -1.839794 | -1.839752 | -1.839735 | -1.839794 | -1.840078 | 0.144326 | 0.144044 | 0.007680 |
| [Ar] $3d^{10}4s^25s^1$ | $^2S$ | -1.883180 | -1.883197 | -1.883209 | -1.883488 | -1.883223 | 0.100631 | 0.100899 | -0.007280 |
| [Ar] $3d^{10}4s^2$ | $^1S$ | -1.783409 | -1.783412 | -1.783411 | -1.783412 | -1.783412 | 0.200707 | 0.200710 | -0.000068 |
| [Ar] $3d^{10}4s^1$ | $^2S$ | -1.093527 | -1.093522 | -1.093520 | -1.093527 | -1.093527 | 0.890593 | 0.890595 | -0.000048 |
| [Ar] $3d^{10}4d^1$ | $^2D$ | -0.462715 | -0.463166 | -0.463207 | -0.463208 | -0.463276 | 1.520912 | 1.520846 | 0.001793 |

TABLE II: K AE gaps and relative errors for various ECPs. All values are in eV

| Gaps | | AE | UC | BFD | MDFSTU | CRENBL | ccECP |
|---|---|---|---|---|---|---|---|
| [Ar] $4s^2$ | $^1S$ | -0.498505 | 0.000354 | -0.001583 | -0.000757 | 0.000433 | -0.000897 |
| [Ar] $4p^1$ | $^2P$ | 1.608079 | 0.000429 | -0.006825 | 0.006632 | -0.002319 | -0.012976 |
| [Ar] $3d^1$ | $^2D$ | 2.669220 | -0.000994 | -0.004400 | 0.013495 | -0.000613 | -0.009866 |
| [Ar] | $^1S$ | 4.326249 | -0.000523 | -0.002396 | 0.010195 | -0.001463 | -0.013438 |
| [Ne] $3s^23p^5$ | $^2P$ | 35.982578 | -0.013839 | -0.025443 | -0.026129 | 0.045011 | 0.039496 |
| [Ne] $3s^23p^4$ | $^3P$ | 81.663324 | -0.055324 | -0.010789 | -0.072645 | 0.035021 | 0.040246 |
| [Ne] $3s^23p^3$ | $^4S$ | 142.428891 | -0.122589 | 0.019629 | -0.144542 | -0.077348 | -0.059660 |
| [Ne] $3s^23p^2$ | $^3P$ | 224.466556 | -0.189978 | 0.325122 | -0.010181 | -0.092057 | -0.039785 |
| [Ne] $3s^23p^1$ | $^2P$ | 323.890212 | -0.291833 | 0.596752 | 0.107788 | -0.276991 | -0.211082 |
| [Ne] $3s^2$ | $^1S$ | 441.570495 | -0.432216 | 0.751372 | 0.183850 | -0.706658 | -0.666719 |
| MAD | | | 0.110808 | 0.174431 | 0.0576214 | 0.123791 | 0.109417 |

## II. POTASSIUM AND CALCIUM

### A. K

In Table II, we show the all electron atomic excitation gaps and relative errors for various ECPs and UC for K atom. In Table III and Table IV, we provide KH and KO AE molecular binding parameters and discrepancies for various core approximations.

TABLE III: KH AE molecular binding parameters and discrepancies for various core approximations. All parameters were obtained using Morse potential fit. The parameters shown are dissociation energy $D_e$, equilibrium bond length $r_e$, vibrational frequency $\omega_e$ and dissociation energy discrepancy at dissociation bond length $D_{diss}$.

| | AE | BFD | CRENBL | MDFSTU | UC | ccECP |
|---|---|---|---|---|---|---|
| $D_e$(eV) | 1.8314(2) | -0.0061(2) | 0.0004(2) | 0.0012(2) | 0.0020(2) | -0.0019(2) |
| $r_e$(Å) | 2.2399(2) | -0.0029(3) | 0.0004(3) | -0.0032(3) | 0.0012(3) | 0.0036(3) |
| $\omega_e$(cm$^{-1}$) | 992.92(32) | 1.40(49) | -0.42(47) | 1.63(49) | -0.87(46) | -0.70(52) |
| $D_{diss}$(eV) | 0 | -0.0223(33) | 0.0015(32) | -0.0131(33) | 0.0073(31) | 0.0201(35) |

### B. Ca

In Table V, we show the all electron atomic excitation gaps and relative errors for various ECPs and UC for Ca atom. In Table VI and Table VII, we provide CaH and CaO AE molecular binding parameters and discrepancies for various core approximations.

TABLE IV: KO AE molecular binding parameters and discrepancies for various core approximations. All parameters were obtained using Morse potential fit. The parameters shown are dissociation energy $D_e$, equilibrium bond length $r_e$, vibrational frequency $\omega_e$ and dissociation energy discrepancy at dissociation bond length $D_{diss}$.

| | AE | BFD | CRENBL | MDFSTU | UC | ccECP |
|---|---|---|---|---|---|---|
| $D_e$(eV) | 2.854(1) | 0.007(2) | 0.006(2) | 0.027(2) | 0.007(2) | -0.002(2) |
| $r_e$(Å) | 2.1665(8) | -0.003(1) | 0.001(1) | -0.002(1) | 0.002(1) | 0.000(1) |
| $\omega_e$(cm$^{-1}$) | 442.77(74) | 0.1(1.0) | -0.2(1.0) | -0.3(1.0) | -0.6(1.0) | 0.9(1.0) |
| $D_{diss}$(eV) | 0 | -0.024(24) | 0.015(24) | 0.005(24) | 0.024(25) | 0.020(24) |

TABLE V: Ca AE gaps and relative errors for various ECPs. All values are in eV

| | | AE | UC | BFD | MDFSTU | CRENBL | ccECP |
|---|---|---|---|---|---|---|---|
| [Ar] $4s^1 4p^1$ | $^3P$ | 1.890174 | 0.001703 | -0.013857 | 0.002887 | -0.001513 | -0.027169 |
| [Ar] $4s^1 3d^1$ | $^3D$ | 2.576290 | 0.006267 | 0.069792 | 0.078317 | 0.013604 | 0.010299 |
| [Ar] $4s^1$ | $^2S$ | 6.103925 | -0.000868 | 0.006526 | 0.015425 | 0.000841 | -0.008007 |
| [Ar] $3d^1$ | $^2D$ | 7.868145 | 0.010700 | 0.097058 | 0.115681 | 0.017358 | 0.005473 |
| [Ar] | $^1S$ | 17.964590 | -0.002868 | 0.002038 | 0.038188 | 0.003251 | -0.041261 |
| [Ne] $3s^2 3p^5$ | $^2P$ | 68.951726 | -0.029271 | -0.015472 | 0.018312 | 0.064218 | 0.009701 |
| [Ne] $3s^2 3p^4$ | $^3P$ | 136.042981 | -0.092184 | -0.010602 | -0.014812 | 0.034262 | 0.013257 |
| [Ne] $3s^2 3p^3$ | $^4S$ | 220.224767 | -0.188033 | -0.013277 | -0.090705 | -0.143938 | -0.076441 |
| [Ne] $3s^2 3p^2$ | $^3P$ | 328.221191 | -0.280149 | 0.291132 | 0.129841 | -0.218807 | 0.044805 |
| [Ne] $3s^2 3p^1$ | $^2P$ | 455.512261 | -0.414993 | 0.538075 | 0.282940 | -0.530014 | 0.005272 |
| [Ne] $3s^2$ | $^1S$ | 602.947774 | -0.597431 | 0.651367 | 0.301606 | -1.166094 | -0.281970 |
| MAD | | | 0.147679 | 0.155381 | 0.0989742 | 0.199446 | 0.047605 |

TABLE VI: CaH AE molecular binding parameters and discrepancies for various core approximations. All parameters were obtained using Morse potential fit. The parameters shown are dissociation energy $D_e$, equilibrium bond length $r_e$, vibrational frequency $\omega_e$ and dissociation energy discrepancy at dissociation bond length $D_{diss}$.

| | AE | BFD | CRENBL | MDFSTU | UC | ccECP |
|---|---|---|---|---|---|---|
| $D_e$(eV) | 1.768(2) | -0.004(3) | 0.002(3) | 0.009(3) | 0.004(3) | -0.019(3) |
| $r_e$(Å) | 2.012(2) | 0.000(3) | 0.000(3) | -0.001(3) | 0.001(3) | -0.000(3) |
| $\omega_e$(cm$^{-1}$) | 1212.3(5.7) | 3.9(8.0) | 0.2(8.1) | 2.2(8.0) | -1.2(8.1) | 4.2(8.0) |
| $D_{diss}$(eV) | 0 | 0.011(43) | 0.005(43) | 0.012(43) | 0.011(43) | -0.011(43) |

TABLE VII: CaO AE molecular binding parameters and discrepancies for various core approximations. All parameters were obtained using Morse potential fit. The parameters shown are dissociation energy $D_e$, equilibrium bond length $r_e$, vibrational frequency $\omega_e$ and dissociation energy discrepancy at dissociation bond length $D_{diss}$.

| | AE | BFD | CRENBL | MDFSTU | UC | ccECP |
|---|---|---|---|---|---|---|
| $D_e$(eV) | 4.145(5) | 0.067(7) | 0.020(7) | 0.081(7) | 0.016(7) | 0.006(7) |
| $r_e$(Å) | 1.830(2) | 0.005(2) | 0.002(2) | 0.004(2) | 0.003(2) | -0.000(2) |
| $\omega_e$(cm$^{-1}$) | 702.3(3.1) | -5.8(4.2) | -1.8(4.3) | -6.3(4.1) | -2.1(4.3) | -1.9(4.3) |
| $D_{diss}$(eV) | 0 | 0.140(91) | 0.055(94) | 0.103(89) | 0.053(94) | -0.028(92) |

## III. GALLIUM - KRYPTON

### A. Ga

In Table VIII, we show the all electron atomic excitation gaps and relative errors for various ECPs and UC for Ga atom. In Table IX and Table X, we provide GaH and GaO AE molecular binding parameters and discrepancies for various core approximations.

TABLE VIII: Gallium AE gaps and relative errors for various ECPs. All values are in eV

| Gaps | | AE | UC | BFD | SDFSTU | MWBSTU | ccECP |
|---|---|---|---|---|---|---|---|
| [Ar] $3d^{10}4s^24p^2$ | $^2P$ | -0.308594 | -0.017786 | -0.040236 | -0.028154 | -0.007378 | -0.022849 |
| [Ar] $3d^{10}4s^14p^2$ | $^4P$ | 4.68977 | -0.361346 | -0.374226 | -0.389590 | -0.378054 | -0.378091 |
| [Ar] $3d^{10}4s^24d^1$ | $^2D$ | 4.23806 | -0.093030 | -0.065598 | -0.068440 | -0.129130 | -0.064934 |
| [Ar] $3d^{10}4s^25s^1$ | $^2S$ | 2.99019 | -0.033639 | 0.024257 | -0.000147 | -0.084836 | -0.002629 |
| [Ar] $3d^{10}4s^2$ | $^1S$ | 5.90688 | -0.068385 | -0.022257 | -0.029745 | -0.103216 | -0.029477 |
| [Ar] $3d^{10}4s^1$ | $^2S$ | 26.3617 | -0.733594 | -0.656568 | -0.654376 | -0.801611 | -0.624231 |
| [Ar] $3d^{10}4d^1$ | $^2D$ | 43.7536 | -1.492386 | -1.038511 | -0.945629 | -1.077799 | -0.864267 |
| MAD | | | 0.400024 | 0.317379 | 0.302297 | 0.368861 | 0.283783 |

TABLE IX: GaH AE molecular binding parameters and discrepancies for various core approximations. All parameters were obtained using Morse potential fit. The parameters shown are dissociation energy $D_e$, equilibrium bond length $r_e$, vibrational frequency $\omega_e$ and dissociation energy discrepancy at dissociation bond length $D_{diss}$.

| | AE | BFD | MDFSTU | SDFSTU | UC | ccECP |
|---|---|---|---|---|---|---|
| $D_e$(eV) | 3.001(7) | -0.07(1) | 0.06(1) | -0.02(1) | -0.00(1) | 0.00(1) |
| $r_e$(Å) | 1.645(4) | -0.004(5) | 0.024(5) | 0.011(5) | -0.002(5) | 0.012(5) |
| $\omega_e$(cm$^{-1}$) | 1757(13) | 1(18) | -88(17) | -33(17) | 3(19) | -42(17) |
| $D_{diss}$(eV) | 0 | -0.16(11) | 0.04(11) | -0.00(11) | -0.02(12) | -0.00(11) |

TABLE X: GaO AE molecular binding parameters and discrepancies for various core approximations. All parameters were obtained using Morse potential fit. The parameters shown are dissociation energy $D_e$, equilibrium bond length $r_e$, vibrational frequency $\omega_e$ and dissociation energy discrepancy at dissociation bond length $D_{diss}$.

| | AE | BFD | MDFSTU | SDFSTU | ccECP |
|---|---|---|---|---|---|
| $D_e$(eV) | 4.28(2) | -0.49(3) | 0.11(3) | -0.07(3) | -0.04(3) |
| $r_e$(Å) | 1.692(4) | -0.053(6) | 0.006(6) | 0.000(6) | 0.004(6) |
| $\omega_e$(cm$^{-1}$) | 806.2(9.9) | 21(15) | -71(14) | -17(13) | -22(14) |
| $D_{diss}$(eV) | 0 | -1.89(20) | -0.66(23) | -0.33(25) | -0.23(26) |

### B. Ge

In Table XI, we show the all electron atomic excitation gaps and relative errors for various ECPs and UC for Ge atom. In Table XII and Table XIII, we provide GeH and GeO AE molecular binding parameters and discrepancies for various core approximations.

### C. As

In Table XIV, we show the all electron atomic excitation gaps and relative errors for various ECPs and UC for As atom. In Table XV and Table XVI, we provide AsH and AsO AE molecular binding parameters and discrepancies for various core approximations.

### D. Se

In Table XVII, we show the all electron atomic excitation gaps and relative errors for various ECPs and UC for Se atom. In Table XVIII and Table XIX, we provide SeH and SeO AE molecular binding parameters and discrepancies for various core approximations.

TABLE XI: Germanium AE gaps and relative errors for various ECPs. All values are in eV

| Gaps | | AE | UC | BFD | SDFSTU | MDFSTU | SBKJC | ccECP |
|---|---|---|---|---|---|---|---|---|
| [Ar] $3d^{10}4s^24p^3$ | $^4S$ | -1.34405 | -0.003518 | -0.021498 | -0.006374 | -0.018903 | 0.016538 | 0.011460 |
| [Ar] $3d^{10}4s^14p^3$ | $^5S$ | 5.07576 | -0.348544 | -0.396305 | -0.418164 | -0.401010 | -0.263160 | -0.411128 |
| [Ar] $3d^{10}4s^24p^1$ | $^2P$ | 7.91209 | -0.077115 | -0.051796 | -0.045754 | -0.050653 | -0.084109 | -0.056692 |
| [Ar] $3d^{10}4s^14p^2$ | $^4P$ | 14.312 | -0.453691 | -0.455459 | -0.481461 | -0.458415 | -0.357605 | -0.486475 |
| [Ar] $3d^{10}4s^24d^1$ | $^2S$ | 16.0441 | -0.747582 | -0.738607 | -0.800014 | -0.778003 | -0.675376 | -0.803107 |
| [Ar] $3d^{10}4s^25s^1$ | $^2S$ | 15.5016 | -0.174770 | -0.143561 | -0.097374 | -0.143156 | -0.196280 | -0.104004 |
| [Ar] $3d^{10}4s^2$ | $^1S$ | 23.695 | -0.254466 | -0.216643 | -0.152026 | -0.206844 | -0.229962 | -0.145338 |
| [Ar] $3d^{10}4s^1$ | $^2S$ | 57.769 | -1.018601 | -0.963409 | -0.853169 | -0.961434 | -0.755071 | -0.767064 |
| [Ar] $3d^{10}4d^1$ | $^2S$ | 81.4436 | -1.800408 | -1.488412 | -1.537638 | -1.692764 | -1.153363 | -1.433766 |
| MAD | | | 0.542077 | 0.497299 | 0.487997 | 0.523465 | 0.414607 | 0.468781 |

TABLE XII: GeH AE molecular binding parameters and discrepancies for various core approximations. All parameters were obtained using Morse potential fit. The parameters shown are dissociation energy $D_e$, equilibrium bond length $r_e$, vibrational frequency $\omega_e$ and dissociation energy discrepancy at dissociation bond length $D_{diss}$.

| | AE | BFD | MDFSTU | SBKJC | SDFSTU | UC | ccECP |
|---|---|---|---|---|---|---|---|
| $D_e$(eV) | 2.948(3) | -0.028(4) | -0.026(4) | 0.021(4) | 0.040(4) | 0.017(4) | 0.037(4) |
| $r_e$(Å) | 1.581(1) | 0.005(2) | 0.004(2) | 0.008(2) | 0.010(2) | 0.015(2) | 0.008(2) |
| $\omega_e$(cm$^{-1}$) | 1954.3(5.8) | -6.6(7.7) | -16.0(7.4) | -41.4(7.3) | -48.2(7.3) | -16.6(8.0) | -49.9(7.1) |
| $D_{diss}$(eV) | 0 | 0.020(44) | -0.029(42) | -0.001(41) | 0.026(41) | 0.221(48) | -0.022(39) |

TABLE XIII: GeO AE molecular binding parameters and discrepancies for various core approximations. All parameters were obtained using Morse potential fit. The parameters shown are dissociation energy $D_e$, equilibrium bond length $r_e$, vibrational frequency $\omega_e$ and dissociation energy discrepancy at dissociation bond length $D_{diss}$.

| | AE | BFD | MDFSTU | SBKJC | SDFSTU | UC | ccECP |
|---|---|---|---|---|---|---|---|
| $D_e$(eV) | 7.018(8) | -0.24(1) | -0.20(1) | -0.09(1) | 0.16(1) | 0.139(8) | 0.071(9) |
| $r_e$(Å) | 1.622(1) | -0.014(1) | -0.014(1) | -0.012(1) | 0.001(1) | 0.024(1) | 0.001(1) |
| $\omega_e$(cm$^{-1}$) | 1020.1(3.4) | 2.5(4.8) | -9.3(4.6) | -28.2(4.4) | -46.3(4.5) | -21.2(3.6) | -44.8(4.1) |
| $D_{diss}$(eV) | 0 | -0.98(11) | -1.15(10) | -1.212(93) | -0.56(10) | 1.09(10) | -0.665(92) |

TABLE XIV: Arsenic AE gaps and relative errors for various ECPs. All values are in eV.

| Gaps | | AE | UC | BFD | SDFSTU | MDFSTU | SBKJC | ccECP |
|---|---|---|---|---|---|---|---|---|
| [Ar] $3d^{10}4s^24p^4$ | $^3P$ | -0.724091 | -0.005014 | 0.012891 | 0.010620 | 0.032005 | 0.027401 | 0.005978 |
| [Ar] $3d^{10}4s^14p^4$ | $^4P$ | 8.35428 | -0.416968 | -0.452066 | -0.465908 | -0.336699 | -0.440932 | -0.374654 |
| [Ar] $3d^{10}4s^24p^2$ | $^3P$ | 10.0084 | -0.070574 | -0.040398 | -0.033818 | -0.221315 | -0.070739 | 0.013975 |
| [Ar] $3d^{10}4s^14p^3$ | $^5S$ | 16.5826 | -0.423966 | -0.483069 | -0.482844 | -0.113718 | -0.488919 | -0.396500 |
| [Ar] $3d^{10}4s^24p^1$ | $^2P$ | 28.6027 | -0.220270 | -0.153227 | -0.070841 | -0.675418 | -0.184908 | -0.015124 |
| [Ar] $3d^{10}4s^2$ | $^1S$ | 56.717 | -0.460710 | -0.373396 | -0.183134 | -1.427130 | -0.338783 | -0.126181 |
| [Ar] $3d^{10}4s^1$ | $^2S$ | 106.535 | -1.250948 | -1.129265 | -0.869508 | -2.272360 | -0.975610 | -0.696567 |
| [Ar] $3d^{10}4d^1$ | $^2D$ | 135.966 | -1.951530 | -1.463639 | -1.502414 | -2.925639 | -1.392788 | -0.593634 |
| MAD | | | 0.599997 | 0.513494 | 0.452386 | 1.000536 | 0.490010 | 0.277827 |

TABLE XV: AsH AE molecular binding parameters and discrepancies for various core approximations. All parameters were obtained using Morse potential fit. The parameters shown are dissociation energy $D_e$, equilibrium bond length $r_e$, vibrational frequency $\omega_e$ and dissociation energy discrepancy at dissociation bond length $D_{diss}$.

| | AE | BFD | MDFSTU | SBKJC | SDFSTU | UC | ccECP |
|---|---|---|---|---|---|---|---|
| $D_e$(eV) | 2.870(2) | 0.008(2) | 0.022(2) | 0.036(2) | -0.002(2) | 0.018(2) | 0.002(2) |
| $r_e$(Å) | 1.5185(6) | 0.0052(8) | 0.0226(8) | 0.0068(9) | 0.0015(9) | 0.0105(8) | 0.0016(8) |
| $\omega_e$(cm$^{-1}$) | 2154.8(3.4) | -17.8(5.0) | -49.2(4.4) | -35.4(5.2) | -7.2(5.1) | -17.0(4.6) | -3.8(5.0) |
| $D_{diss}$(eV) | 0 | 0.047(25) | 0.294(23) | 0.052(26) | -0.001(25) | 0.172(24) | 0.021(25) |

TABLE XVI: AsO AE molecular binding parameters and discrepancies for various core approximations. All parameters were obtained using Morse potential fit. The parameters shown are dissociation energy $D_e$, equilibrium bond length $r_e$, vibrational frequency $\omega_e$ and dissociation energy discrepancy at dissociation bond length $D_{diss}$.

| | AE | BFD | MDFSTU | SBKJC | SDFSTU | UC | ccECP |
|---|---|---|---|---|---|---|---|
| $D_e$(eV) | 4.907(5) | -0.071(8) | -0.133(6) | -0.016(8) | -0.100(8) | 0.028(7) | -0.032(7) |
| $r_e$(Å) | 1.6192(8) | -0.004(1) | 0.005(1) | -0.003(1) | -0.010(1) | 0.011(1) | -0.002(1) |
| $\omega_e$(cm$^{-1}$) | 965.9(2.3) | -6.7(3.6) | -7.7(3.0) | -21.3(3.9) | 2.8(3.7) | -7.7(3.1) | -0.9(3.4) |
| $D_{diss}$(eV) | 0 | -0.354(66) | -0.098(58) | -0.425(70) | -0.522(66) | 0.399(64) | -0.142(65) |

TABLE XVII: Selenium AE gaps and relative errors for various ECPs. All values are in eV

| Gaps | | AE | UC | BFD | SDFSTU | MDFSTU | SBKJC | ccECP |
|---|---|---|---|---|---|---|---|---|
| [Ar] $3d^{10}4s^24p^5$ | $^2P$ | -2.04709 | 0.004416 | 0.017297 | 0.001337 | 0.016420 | 0.033244 | -0.006921 |
| [Ar] $3d^{10}4s^14p^5$ | $^3P$ | 9.58661 | -0.559848 | -0.475727 | -0.499457 | -0.541504 | -0.507026 | -0.449462 |
| [Ar] $3d^{10}4s^24p^35s^1$ | $^5S$ | 5.86081 | 1.282282 | -0.104724 | -0.031367 | -0.069982 | -0.110486 | -0.001286 |
| [Ar] $3d^{10}4s^24p^34d^1$ | $^5S$ | 7.75271 | -0.081383 | -0.123423 | -0.085663 | -0.125883 | -0.133500 | -0.037433 |
| [Ar] $3d^{10}4s^24p^3$ | $^4S$ | 9.63653 | -0.064706 | -0.101163 | -0.048144 | -0.085372 | -0.109980 | -0.031353 |
| [Ar] $3d^{10}4s^14p^4$ | $^4P$ | 20.2879 | -0.384795 | -0.497887 | -0.451573 | -0.476280 | -0.470758 | -0.497084 |
| [Ar] $3d^{10}4s^24p^2$ | $^3P$ | 31.1547 | -0.190478 | -0.183543 | -0.033352 | -0.160622 | -0.215235 | 0.016033 |
| [Ar] $3d^{10}4s^24p^1$ | $^2P$ | 62.8487 | -0.392899 | -0.347295 | -0.053809 | -0.294392 | -0.374534 | 0.038396 |
| [Ar] $3d^{10}4s^24d^1$ | $^2P$ | 81.0816 | 0.031123 | 0.276014 | 0.468211 | 0.133466 | 0.151523 | 0.830263 |
| [Ar] $3s^{10}4s^2$ | $^1S$ | 105.494 | -0.681437 | -0.631455 | -0.139423 | -0.504270 | -0.593189 | 0.005228 |
| [Ar] $3d^{10}4s^1$ | $^2S$ | 173.123 | -1.496694 | -1.424434 | -0.805356 | -1.279690 | -1.286627 | -0.776257 |
| [Ar] $3d^{10}4d^1$ | $^2S$ | 208.272 | -2.128374 | -1.204680 | -1.371057 | -1.908936 | -1.663520 | -1.002600 |
| MAD | | | 0.608203 | 0.448970 | 0.332396 | 0.466401 | 0.470802 | 0.307693 |

TABLE XVIII: SeH AE molecular binding parameters and discrepancies for various core approximations. All parameters were obtained using Morse potential fit. The parameters shown are dissociation energy $D_e$, equilibrium bond length $r_e$, vibrational frequency $\omega_e$ and dissociation energy discrepancy at dissociation bond length $D_{diss}$.

| | AE | BFD | MDFSTU | SBKJC | SDFSTU | UC | ccECP |
|---|---|---|---|---|---|---|---|
| $D_e$(eV) | 3.374(1) | 0.020(1) | 0.005(1) | 0.037(1) | -0.019(1) | 0.024(1) | 0.009(1) |
| $r_e$(Å) | 1.4609(3) | 0.0055(5) | 0.0022(5) | 0.0055(5) | -0.0020(5) | 0.0077(5) | 0.0009(5) |
| $\omega_e$(cm$^{-1}$) | 2417.0(2.3) | -13.4(3.2) | -11.8(3.2) | -28.9(3.2) | 5.3(3.2) | -15.3(3.2) | -6.3(3.2) |
| $D_{diss}$(eV) | 0 | 0.108(17) | 0.013(17) | 0.070(17) | -0.053(17) | 0.160(18) | 0.009(17) |

TABLE XIX: SeO AE molecular binding parameters and discrepancies for various core approximations. All parameters were obtained using Morse potential fit. The parameters shown are dissociation energy $D_e$, equilibrium bond length $r_e$, vibrational frequency $\omega_e$ and dissociation energy discrepancy at dissociation bond length $D_{diss}$.

| | AE | BFD | MDFSTU | SBKJC | SDFSTU | UC | ccECP |
|---|---|---|---|---|---|---|---|
| $D_e$(eV) | 4.503(7) | -0.047(9) | -0.12(1) | -0.04(1) | -0.14(1) | 0.010(9) | 0.01(1) |
| $r_e$(Å) | 1.632(1) | 0.001(2) | -0.010(2) | -0.001(2) | -0.014(2) | 0.007(2) | 0.001(2) |
| $\omega_e$(cm$^{-1}$) | 925.5(4.1) | 0.7(5.3) | 3.5(5.5) | -9.7(5.7) | 13.2(5.6) | -6.2(5.2) | -7.0(5.6) |
| $D_{diss}$(eV) | 0 | -0.017(96) | -0.501(91) | -0.237(97) | -0.549(92) | 0.214(97) | -0.06(10) |

### E. Br

In Table XX, we show the all electron atomic excitation gaps and relative errors for various ECPs and UC for Br atom. In Table XXI and Table XXII, we provide BrH and BrO AE molecular binding parameters and discrepancies for various core approximations.

TABLE XX: Bromine AE gaps and relative errors for various ECPs. All values are in eV

| Gaps | | AE | UC | BFD | SDFSTU | MDFSTU | SBKJC | ccECP |
|---|---|---|---|---|---|---|---|---|
| [Ar] $3d^{10}4s^24p^6$ | $^1S$ | -3.5302 | 0.008387 | -0.010772 | 0.015685 | 0.011078 | 0.029656 | -0.045779 |
| [Ar] $3d^{10}4s^14p^6$ | $^2S$ | 10.7639 | -0.500222 | -0.637369 | -0.547524 | -0.506594 | -0.510995 | -0.371900 |
| [Ar] $3d^{10}4s^24p^4$ | $^3P$ | 11.8996 | -0.060199 | -0.035862 | -0.076645 | -0.080008 | -0.090214 | 0.009181 |
| [Ar] $3d^{10}4s^14p^5$ | $^3P$ | 24.0318 | -0.351589 | -0.469121 | -0.530361 | -0.461619 | -0.498083 | -0.318104 |
| [Ar] $3d^{10}4s^24p^35s^1$ | $^5S$ | 23.4013 | -0.148855 | -0.139215 | -0.233650 | -0.286420 | -0.254729 | 0.001823 |
| [Ar] $3d^{10}4s^24p^34d^1$ | $^5D$ | 24.6519 | -0.213290 | -0.530144 | -0.390964 | -0.308298 | -0.327592 | -0.001103 |
| [Ar] $3d^{10}4s^24p^3$ | $^4S$ | 33.3507 | -0.184161 | -0.144446 | -0.233417 | -0.254545 | -0.250109 | -0.053099 |
| [Ar] $3d^{10}4s^24p^2$ | $^3P$ | 68.7533 | -0.353737 | -0.176469 | -0.317566 | -0.355017 | -0.350375 | -0.039465 |
| [Ar] $3d^{10}4s^24p^1$ | $^2P$ | 115.734 | -0.598083 | -0.291302 | -0.476530 | -0.549506 | -0.500139 | -0.142567 |
| [Ar] $3d^{10}4s^24d^1$ | $^2D$ | 138.312 | -0.280207 | -0.210776 | -0.165543 | 0.061847 | -0.044695 | 0.733894 |
| [Ar] $3s^{10}4s^2$ | $^1S$ | 174.976 | -0.926212 | -0.528458 | -0.742365 | -0.880048 | -0.712592 | -0.421401 |
| [Ar] $3d^{10}4s^1$ | $^2S$ | 262.411 | -1.767388 | -1.197872 | -1.575162 | -1.672510 | -1.488942 | -1.410461 |
| [Ar] $3d^{10}4d^1$ | $^2D$ | 303.258 | -2.333763 | -1.762506 | -2.141028 | -1.300857 | -1.869432 | -0.951208 |
| MAD | | | 0.594315 | 0.471870 | 0.572803 | 0.517565 | 0.532889 | 0.346153 |

TABLE XXI: BrH AE molecular binding parameters and discrepancies for various core approximations. All parameters were obtained using Morse potential fit. The parameters shown are dissociation energy $D_e$, equilibrium bond length $r_e$, vibrational frequency $\omega_e$ and dissociation energy discrepancy at dissociation bond length $D_{diss}$.

| | AE | BFD | MDFSTU | SBKJC | SDFSTU | UC | ccECP |
|---|---|---|---|---|---|---|---|
| $D_e$(eV) | 4.054(3) | 0.016(4) | 0.008(4) | 0.031(4) | -0.076(4) | 0.028(4) | -0.027(4) |
| $r_e$(Å) | 1.4099(5) | 0.0036(7) | 0.0010(7) | 0.0029(7) | -0.0052(7) | 0.0058(7) | 0.0005(7) |
| $\omega_e$(cm$^{-1}$) | 2692.3(3.8) | -10.1(5.3) | -11.5(5.3) | -19.7(5.3) | 30.0(5.3) | -13.9(5.3) | 4.5(5.3) |
| $D_{diss}$(eV) | 0 | 0.085(30) | -0.008(30) | 0.044(30) | -0.133(29) | 0.152(31) | -0.004(30) |

TABLE XXII: BrO AE molecular binding parameters and discrepancies for various core approximations. All parameters were obtained using Morse potential fit. The parameters shown are dissociation energy $D_e$, equilibrium bond length $r_e$, vibrational frequency $\omega_e$ and dissociation energy discrepancy at dissociation bond length $D_{diss}$.

| | AE | BFD | MDFSTU | SBKJC | SDFSTU | UC | ccECP |
|---|---|---|---|---|---|---|---|
| $D_e$(eV) | 2.445(2) | -0.021(3) | -0.043(3) | -0.018(3) | -0.248(2) | 0.002(2) | -0.007(3) |
| $r_e$(Å) | 1.7173(7) | -0.0013(9) | -0.009(1) | -0.004(1) | -0.0417(8) | 0.0048(9) | 0.000(1) |
| $\omega_e$(cm$^{-1}$) | 704.6(1.7) | 4.4(2.4) | 3.3(2.5) | -0.7(2.5) | 46.3(2.3) | -2.5(2.3) | -1.1(2.5) |
| $D_{diss}$(eV) | 0 | -0.016(31) | -0.223(30) | -0.110(31) | -0.795(24) | 0.084(31) | -0.016(32) |

### F. Kr

In Table XXIII, we show the all electron atomic excitation gaps and relative errors for various ECPs and UC for Kr atom. In Table XXIV, we provide $KrH^+$ AE molecular binding parameters and discrepancies for various core approximations.

## IV. ADDITIONAL PSEUDOPOTENTIALS

### A. H

In Table XXV, we provide $H_2$ AE molecular binding parameters and discrepancies for various core approximations.

### B. He

In Table XXVI, we provide $HeH^+$ AE molecular binding parameters and discrepancies for various core approximations.

TABLE XXIII: Krypton AE gaps and relative errors for various ECPs. All values are in eV

| Gaps | | AE | UC | BFD | MWBSTU | SBKJC | ccECP |
|---|---|---|---|---|---|---|---|
| [Ar] $3d^{10}4s^2 4p^5 5s^1$ | $^3P$ | 10.1426 | -0.038341 | -0.018153 | -0.063355 | -0.073100 | 0.021594 |
| [Ar] $3d^{10}4s^2 4p^5$ | $^2P$ | 14.2209 | -0.048091 | -0.026997 | -0.059340 | -0.071471 | 0.040846 |
| [Ar] $3d^{10}4s^2 4p^4$ | $^3P$ | 38.6728 | -0.150398 | -0.105340 | -0.184130 | -0.204095 | 0.051657 |
| [Ar] $3d^{10}4s^2 4p^3 4d^1$ | $^5D$ | 55.608 | -0.329969 | -0.212654 | -0.238547 | -0.534719 | -0.052178 |
| [Ar] $3d^{10}4s^2 4p^3$ | $^4S$ | 74.2656 | -0.316318 | -0.257432 | -0.398686 | -0.412952 | -0.000527 |
| [Ar] $3d^{10}4s^2 4p^2$ | $^3P$ | 125.685 | -0.513349 | -0.282396 | -0.465859 | -0.522160 | 0.103625 |
| [Ar] $3d^{10}4s^2 4p^1$ | $^2P$ | 189.984 | -0.783442 | -0.388464 | -0.626898 | -0.696714 | 0.105656 |
| [Ar] $3d^{10}4s^2 4d^1$ | $^2D$ | 216.765 | -0.513080 | 0.490381 | 0.369630 | -0.304375 | 0.827956 |
| [Ar] $3s^{10}4s^2$ | $^1S$ | 267.782 | -1.135023 | -0.614504 | -0.928820 | -0.956408 | -0.049760 |
| [Ar] $3d^{10}4s^1$ | $^2S$ | 376.952 | -1.986150 | -1.533119 | -1.754401 | -1.841830 | 0.057466 |
| [Ar] $3d^{10}4d^1$ | $^2D$ | 423.489 | -2.501284 | -0.921242 | -0.873884 | -2.259004 | 0.827080 |
| MAD | | | 0.755949 | 0.440971 | 0.542141 | 0.716075 | 0.194395 |

TABLE XXIV: $KrH^+$ AE molecular binding parameters and discrepancies for various core approximations. All parameters were obtained using Morse potential fit. The parameters shown are dissociation energy $D_e$, equilibrium bond length $r_e$, vibrational frequency $\omega_e$ and dissociation energy discrepancy at dissociation bond length $D_{diss}$.

| | AE | BFD | MDFSTU | SBKJC | UC | ccECP |
|---|---|---|---|---|---|---|
| $D_e$(eV) | 4.60(1) | 0.01(2) | -0.00(2) | -0.02(2) | -0.01(2) | 0.02(2) |
| $r_e$(Å) | 1.422(3) | 0.004(4) | 0.001(4) | 0.002(4) | 0.004(4) | -0.002(4) |
| $\omega_e$(cm$^{-1}$) | 2635(20) | -13(27) | -5(28) | -9(28) | -2(28) | -4(27) |
| $D_{diss}$(eV) | 0 | 0.08(17) | -0.01(17) | 0.00(17) | 0.10(18) | -0.05(17) |

TABLE XXV: $H_2$ AE molecular binding parameters and discrepancies for various core approximations. All parameters were obtained using Morse potential fit. The parameters shown are dissociation energy $D_e$, equilibrium bond length $r_e$, vibrational frequency $\omega_e$ and dissociation energy discrepancy at dissociation bond length $D_{diss}$.

| | AE | BFD | ccECP | eCEPP |
|---|---|---|---|---|
| $D_e$(eV) | 4.76(1) | -0.03(2) | -0.00(2) | 0.00(2) |
| $r_e$(Å) | 0.736(3) | -0.009(4) | 0.000(4) | -0.000(4) |
| $\omega_e$(cm$^{-1}$) | 4768(53) | 46(86) | -0(75) | -1(75) |
| $D_{diss}$(eV) | 0 | -0.28(28) | -0.00(26) | -0.00(26) |

TABLE XXVI: $HeH^+$ AE molecular binding parameters and discrepancies for various core approximations. All parameters were obtained using Morse potential fit. The parameters shown are dissociation energy $D_e$, equilibrium bond length $r_e$, vibrational frequency $\omega_e$ and dissociation energy discrepancy at dissociation bond length $D_{diss}$.

| | AE | BFD | ccECP |
|---|---|---|---|
| $D_e$(eV) | 2.045(5) | 0.006(7) | 0.001(7) |
| $r_e$(Å) | 0.770(2) | 0.000(2) | 0.000(2) |
| $\omega_e$(cm$^{-1}$) | 3377(23) | -8(32) | -1(32) |
| $D_{diss}$(eV) | 0 | 0.006(76) | 0.002(76) |

### C. Li

In Table XXVII, we show the all electron atomic excitation gaps and relative errors for various ECPs and UC for Li atom. In Table XXVIII and Table XXIX, we provide $Li_2$ and LiO AE molecular binding parameters and discrepancies for various core approximations.

### D. Be

In Table XXX, we show the all electron atomic excitation gaps and relative errors for various ECPs and UC for Be atom. In Table XXXI and Table XXXII, we provide $Be_2$ and BeO AE molecular binding parameters and discrepancies

TABLE XXVII: Li AE gaps and relative errors for various ECPs. All values are in eV

| | AE | UC | BFD | SDFSTU | eCEPP | SBKJC | CRENBL | ccECP | ccECP(reg) |
|---|---|---|---|---|---|---|---|---|---|
| [He]$2s^2$ $^1S$ | -0.617117 | -0.000385 | -0.009589 | -0.009021 | -0.007589 | -0.008405 | -0.009683 | -0.006782 | 0.000022 |
| [He] $^1S$ | 5.391456 | -0.049173 | -0.049159 | -0.057029 | -0.061737 | -0.048485 | -0.045454 | -0.034821 | -0.000149 |
| [He]$2p^1$ $^2P$ | 1.848040 | -0.006615 | -0.006424 | -0.013423 | -0.007934 | -0.006671 | -0.002466 | 0.024668 | 0.001369 |
| [He]$3d^1$ $^2D$ | 3.881222 | -0.047834 | -0.047942 | -0.055524 | -0.060232 | -0.047265 | -0.044313 | -0.033573 | -0.000139 |
| MAD | | 0.0260016 | 0.0282785 | 0.033749 | 0.0343729 | 0.0277064 | 0.0254791 | 0.024961 | 0.000420 |

TABLE XXVIII: $Li_2$ AE molecular binding parameters and discrepancies for various core approximations. All parameters were obtained using Morse potential fit. The parameters shown are dissociation energy $D_e$, equilibrium bond length $r_e$, vibrational frequency $\omega_e$ and dissociation energy discrepancy at dissociation bond length $D_{diss}$.

| | AE | BFD | CRENBL | SBKJC | SDFSTU | UC | ccECP | ccECP-reg | eCEPP |
|---|---|---|---|---|---|---|---|---|---|
| $D_e$(eV) | 1.0500(4) | -0.0069(5) | -0.0076(5) | -0.0046(5) | -0.0038(5) | 0.0063(6) | 0.0018(5) | 0.0004(6) | 0.0040(6) |
| $r_e$(Å) | 2.685(2) | 0.006(3) | 0.004(3) | 0.004(3) | 0.011(3) | 0.025(3) | 0.005(3) | 0.000(3) | 0.020(3) |
| $\omega_e$(cm$^{-1}$) | 334.2(1.3) | -4.2(1.7) | -3.7(1.7) | -4.5(1.8) | -5.6(1.7) | -5.6(1.8) | -4.6(1.7) | -0.1(1.8) | -7.8(1.7) |
| $D_{diss}$(eV) | 0 | -0.027(17) | -0.029(17) | -0.031(17) | -0.015(17) | 0.046(19) | -0.020(17) | 0.001(18) | 0.006(18) |

TABLE XXIX: LiO AE molecular binding parameters and discrepancies for various core approximations. All parameters were obtained using Morse potential fit. The parameters shown are dissociation energy $D_e$, equilibrium bond length $r_e$, vibrational frequency $\omega_e$ and dissociation energy discrepancy at dissociation bond length $D_{diss}$.

| | AE | BFD | CRENBL | SBKJC | SDFSTU | UC | ccECP | ccECP-reg | eCEPP |
|---|---|---|---|---|---|---|---|---|---|
| $D_e$(eV) | 3.34(1) | -0.02(1) | -0.06(1) | -0.03(1) | 0.02(1) | 0.04(1) | 0.03(1) | 0.01(1) | 0.08(1) |
| $r_e$(Å) | 1.581(4) | -0.015(5) | -0.023(5) | -0.020(5) | 0.002(5) | 0.013(6) | -0.006(5) | -0.000(6) | 0.016(5) |
| $\omega_e$(cm$^{-1}$) | 942(10) | -57(12) | -43(13) | -54(13) | -41(13) | -6(15) | -54(12) | 0(15) | -77(12) |
| $D_{diss}$(eV) | 0 | -0.80(12) | -0.86(13) | -0.86(13) | -0.31(15) | 0.27(20) | -0.56(13) | 0.01(19) | -0.33(13) |

for various core approximations.

TABLE XXX: Be AE gaps and relative errors for various ECPs. All values are in eV

| | AE | UC | BFD | SDFSTU | eCEPP | SBKJC | CRENBL | ccECP | ccECP(reg) |
|---|---|---|---|---|---|---|---|---|---|
| [He]$2s^1$ $^2S$ | 9.321170 | -0.020915 | 0.047047 | 0.058307 | 0.027327 | 0.040991 | 0.041970 | 0.039719 | 0.000863 |
| [He] $^1S$ | 27.532207 | -0.104122 | -0.044908 | -0.023159 | -0.112056 | -0.063886 | -0.057119 | -0.045365 | 0.002418 |
| [He]$2p^1$ $^2P$ | 2.724923 | 0.009394 | 0.023031 | 0.019647 | 0.005026 | 0.012395 | 0.037405 | 0.006430 | 0.003561 |
| [He]$3d^1$ $^2D$ | 7.704038 | -0.022045 | 0.044432 | 0.055688 | 0.023563 | 0.037943 | 0.039429 | 0.037199 | 0.000948 |
| MAD | | 0.039119 | 0.0398546 | 0.0392001 | 0.041993 | 0.0388036 | 0.0439809 | 0.0321781 | 0.0019476 |

TABLE XXXI: $Be_2$ AE molecular binding parameters and discrepancies for various core approximations. All parameters were obtained using Morse potential fit. The parameters shown are dissociation energy $D_e$, equilibrium bond length $r_e$, vibrational frequency $\omega_e$ and dissociation energy discrepancy at dissociation bond length $D_{diss}$.

| | AE | BFD | CRENBL | SBKJC | SDFSTU | UC | ccECP | ccECP-reg | eCEPP |
|---|---|---|---|---|---|---|---|---|---|
| $D_e$(eV) | 0.0731(6) | 0.0069(9) | 0.0078(9) | 0.0018(9) | -0.0002(9) | 0.0064(9) | 0.0018(9) | 0.0009(9) | 0.0128(9) |
| $r_e$(Å) | 2.483(5) | 0.008(8) | 0.016(8) | -0.004(8) | -0.016(8) | 0.032(8) | -0.006(8) | 0.004(8) | 0.034(8) |
| $\omega_e$(cm$^{-1}$) | 217.0(3.5) | -8.6(4.9) | -11.1(4.8) | -1.0(5.0) | 3.7(5.1) | -12.8(4.8) | -0.6(5.1) | -2.0(4.9) | -19.3(4.9) |
| $D_{diss}$(eV) | 0 | 0.0072(69) | 0.0110(70) | -0.0012(67) | -0.0076(64) | 0.0182(76) | -0.0022(67) | 0.0017(68) | 0.0220(78) |

### E. F

In Table XXXIII, we show the all electron atomic excitation gaps and relative errors for various ECPs and UC for F atom. In Table XXXIV and Table XXXV, we provide FH and $F_2$ AE molecular binding parameters and discrepancies

TABLE XXXII: BeO AE molecular binding parameters and discrepancies for various core approximations. All parameters were obtained using Morse potential fit. The parameters shown are dissociation energy $D_e$, equilibrium bond length $r_e$, vibrational frequency $\omega_e$ and dissociation energy discrepancy at dissociation bond length $D_{diss}$.

| | AE | BFD | CRENBL | SBKJC | SDFSTU | UC | ccECP | ccECP-reg | eCEPP |
|---|---|---|---|---|---|---|---|---|---|
| $D_e$(eV) | 4.516(3) | 0.101(4) | 0.076(4) | 0.042(4) | 0.040(4) | 0.064(4) | 0.042(4) | 0.013(4) | 0.187(4) |
| $r_e$(Å) | 1.3327(6) | 0.001(1) | -0.001(1) | -0.005(1) | -0.004(1) | 0.0060(9) | -0.005(1) | -0.0005(9) | 0.004(1) |
| $\omega_e$(cm$^{-1}$) | 1445.9(3.6) | -44.1(6.5) | -32.4(6.0) | -29.4(5.7) | -20.5(5.7) | -13.7(5.0) | -31.6(6.2) | 0.6(5.2) | -86.3(5.9) |
| $D_{diss}$(eV) | 0 | -0.191(69) | -0.221(63) | -0.389(59) | -0.287(60) | 0.212(58) | -0.385(64) | 0.006(58) | -0.304(60) |

for various core approximations.

TABLE XXXIII: F AE gaps and relative errors for various ECPs. All values are in eV

| | | AE | UC | BFD | MWBSTU | SDFSTU | eCEPP | SBKJC | CRENBL | ccECP |
|---|---|---|---|---|---|---|---|---|---|---|
| [He]$2s^2 2p^6$ | $^1S$ | -3.399708 | 0.004137 | 0.009719 | 0.016332 | 0.037166 | -0.001574 | -0.005987 | -0.001712 | 0.005463 |
| [He]$2s^2 2p^4 3s^1$ | $^4P$ | 12.671376 | -0.017130 | -0.090711 | -0.002002 | -0.043657 | -0.008253 | -0.009045 | -0.014050 | -0.032083 |
| [He]$2s^2 2p^4$ | $^3P$ | 42.438405 | -0.039091 | -0.112786 | 0.029755 | 0.014277 | -0.014056 | -0.008144 | -0.008331 | 0.002200 |
| [He]$2s^2 2p^3 3p^1$ | $^5P$ | 45.978897 | -0.043831 | -0.118159 | 0.030851 | 0.008738 | -0.007327 | -0.004845 | -0.006689 | -0.004585 |
| [He]$2s^2 2p^3 3d^1$ | $^5D$ | 17.391794 | -0.014858 | -0.038801 | -0.001361 | -0.018281 | -0.004656 | -0.001948 | -0.004375 | -0.005070 |
| [He]$2s^2 2p^3$ | $^4S$ | 52.297032 | -0.043128 | -0.118745 | 0.054320 | 0.024255 | -0.007021 | -0.003324 | -0.005624 | -0.005189 |
| [He]$2s^2 2p^2$ | $^3P$ | 115.047978 | -0.107110 | -0.275577 | 0.208120 | 0.180048 | 0.013303 | -0.025577 | -0.024715 | -0.000296 |
| [He]$2s^2 2p^1$ | $^2P$ | 202.222480 | -0.198487 | -0.566032 | 0.532155 | 0.466679 | 0.052232 | -0.038028 | -0.038965 | -0.033479 |
| [He]$2s^2$ | $^1S$ | 316.393981 | -0.323729 | -1.072021 | 1.079635 | 0.895938 | 0.084630 | -0.043674 | -0.058545 | -0.165068 |
| MAD | | | 0.0879447 | 0.26695 | 0.21717 | 0.187671 | 0.0214504 | 0.0156192 | 0.0181117 | 0.0281593 |

TABLE XXXIV: FH AE molecular binding parameters and discrepancies for various core approximations. All parameters were obtained using Morse potential fit. The parameters shown are dissociation energy $D_e$, equilibrium bond length $r_e$, vibrational frequency $\omega_e$ and dissociation energy discrepancy at dissociation bond length $D_{diss}$.

| | AE | BFD | CRENBL | MDFSTU | SBKJC | SDFSTU | UC | ccECP | eCEPP |
|---|---|---|---|---|---|---|---|---|---|
| $D_e$(eV) | 6.15(1) | 0.02(2) | 0.01(2) | 0.03(2) | 0.01(2) | 0.03(2) | 0.01(2) | 0.01(2) | 0.02(2) |
| $r_e$(Å) | 0.915(2) | 0.001(3) | 0.001(3) | 0.000(3) | 0.001(3) | -0.001(3) | 0.001(3) | -0.000(3) | 0.001(3) |
| $\omega_e$(cm$^{-1}$) | 4379(36) | -12(51) | -8(51) | -9(51) | -7(51) | -12(51) | -4(51) | -6(51) | -7(51) |
| $D_{diss}$(eV) | 0 | 0.02(25) | 0.03(25) | 0.01(25) | 0.05(25) | -0.05(25) | 0.03(25) | -0.03(25) | 0.04(25) |

TABLE XXXV: $F_2$ AE molecular binding parameters and discrepancies for various core approximations. All parameters were obtained using Morse potential fit. The parameters shown are dissociation energy $D_e$, equilibrium bond length $r_e$, vibrational frequency $\omega_e$ and dissociation energy discrepancy at dissociation bond length $D_{diss}$.

| | AE | BFD | CRENBL | MDFSTU | SBKJC | SDFSTU | UC | ccECP | eCEPP |
|---|---|---|---|---|---|---|---|---|---|
| $D_e$(eV) | 1.645(4) | -0.010(5) | 0.014(5) | -0.062(5) | 0.015(5) | -0.062(5) | -0.003(5) | -0.002(5) | 0.027(5) |
| $r_e$(Å) | 1.411(2) | 0.000(3) | 0.004(3) | -0.001(3) | 0.004(3) | -0.001(3) | 0.002(3) | 0.002(3) | 0.005(3) |
| $\omega_e$(cm$^{-1}$) | 872.4(9.1) | 2(13) | -6(13) | 6(12) | -6(13) | 7(13) | -2(13) | -1(13) | -9(13) |
| $D_{diss}$(eV) | 0 | 0.007(85) | 0.057(87) | -0.069(81) | 0.059(86) | -0.072(82) | 0.017(85) | 0.023(86) | 0.079(87) |

### F. Ne

In Table XXXVI, we show the all electron atomic excitation gaps and relative errors for various ECPs and UC for Ne atom. In Table XXXVII, we provide $NeH^+$ AE molecular binding parameters and discrepancies for various core approximations.

TABLE XXXVI: Ne AE gaps and relative errors for various ECPs. All values are in eV

| | | AE | UC | BFD | MWBSTU | SBKJC | CRENBL | ccECP |
|---|---|---|---|---|---|---|---|---|
| [He]$2s^2 2p^5 3s^1$ | $^3P$ | 16.628410 | -0.016490 | -0.068427 | -0.034761 | 0.010277 | -0.000719 | -0.024392 |
| [He]$2s^2 2p^5$ | $^2P$ | 21.568150 | -0.014743 | -0.027608 | -0.026732 | 0.008993 | 0.002559 | -0.002497 |
| [He]$2s^2 2p^4$ | $^3P$ | 62.498592 | -0.040624 | -0.083702 | -0.027542 | 0.019612 | 0.010522 | 0.001519 |
| [He]$2s^2 2p^3 3p^1$ | $^5P$ | 105.625302 | -0.072554 | -0.190670 | -0.017268 | 0.033695 | 0.029768 | 0.010843 |
| [He]$2s^2 2p^3 3d^1$ | $^5D$ | 111.361128 | -0.081446 | -0.164414 | -0.126928 | 0.042545 | 0.035398 | 0.022803 |
| [He]$2s^2 2p^3$ | $^4S$ | 125.833191 | -0.079920 | -0.178068 | 0.038484 | 0.047136 | 0.038228 | 0.017994 |
| [He]$2s^2 2p^2$ | $^3P$ | 223.123150 | -0.156395 | -0.333163 | 0.190535 | 0.054335 | 0.051296 | 0.035164 |
| [He]$2s^2 2p^1$ | $^2P$ | 349.416322 | -0.259825 | -0.639356 | 0.489633 | 0.075299 | 0.074574 | 0.020203 |
| [He]$2s^2$ | $^1S$ | 507.238260 | -0.396263 | -1.195806 | 0.961679 | 0.095800 | 0.088753 | -0.080539 |
| MAD | | | 0.124251 | 0.320135 | 0.212618 | 0.043077 | 0.0368685 | 0.023995 |

TABLE XXXVII: $NeH^+$ AE molecular binding parameters and discrepancies for various core approximations. All parameters were obtained using Morse potential fit. The parameters shown are dissociation energy $D_e$, equilibrium bond length $r_e$, vibrational frequency $\omega_e$ and dissociation energy discrepancy at dissociation bond length $D_{diss}$.

| | AE | BFD | CRENBL | MDFSTU | SBKJC | UC | ccECP |
|---|---|---|---|---|---|---|---|
| $D_e$(eV) | 2.309(6) | 0.006(8) | 0.008(8) | -0.014(8) | 0.010(8) | -0.003(8) | 0.007(8) |
| $r_e$(Å) | 0.987(2) | 0.001(2) | 0.001(2) | -0.001(2) | 0.001(2) | 0.000(2) | 0.000(2) |
| $\omega_e$(cm$^{-1}$) | 3056(20) | -8(28) | -7(28) | 8(28) | -6(28) | -0(28) | -7(28) |
| $D_{diss}$(eV) | 0 | 0.019(82) | 0.019(82) | -0.034(81) | 0.026(82) | 0.004(82) | 0.008(81) |

### G. Multiplets of Ge and Se

In tables XXXVIII and XXXIX, we show the multiplet splitting gaps from $^3P$ ground state for Ge and Se respectively. The energies are calculated with FCI and nearly exact CIPSI+PT2 methods correspondingly.

TABLE XXXVIII: Germanium multiplet splitting gaps [eV] from $^3$P ground state. Errors of various core approximations are shown relative to the experiment [1]. FCI with aug-cc-pVQZ basis set.

| Gaps | | Expt. | UC | BFD | MDFSTU | SDFSTU | SBKJC | ccECP |
|---|---|---|---|---|---|---|---|---|
| [Ar] $3d^{10}4s^24p^2$ | $^3P$ | 0.000000 | | | | | | |
| [Ar] $3d^{10}4s^24p^2$ | $^1D$ | 0.883424 | -0.123125 | -0.112430 | -0.112879 | -0.110551 | -0.119385 | -0.111619 |
| [Ar] $3d^{10}4s^24p^2$ | $^1S$ | 2.029291 | -0.123972 | -0.110073 | -0.106829 | -0.106534 | -0.121995 | -0.110102 |
| MAD | | | 0.123548 | 0.111252 | 0.109854 | 0.108542 | 0.12069 | 0.11086 |

TABLE XXXIX: Selenium multiplet splitting gaps [eV] from $^3$P ground state. Errors of various core approximations are shown relative to the experiment [1]. CIPSI+PT2 ($\sim$ 300K dets) with aug-cc-pVQZ basis set.

| Gaps | | Expt. | BFD | MDFSTU | SDFSTU | SBKJC | ccECP |
|---|---|---|---|---|---|---|---|
| [Ar] $3d^{10}4s^24p^4$ | $^3P$ | 0.000000 | | | | | |
| [Ar] $3d^{10}4s^24p^4$ | $^1D$ | 1.187291 | -0.105809 | -0.110100 | 0.048543 | -0.115042 | -0.099090 |
| [Ar] $3d^{10}4s^24p^4$ | $^1S$ | 2.782974 | -0.099501 | -0.108308 | 0.061715 | -0.110258 | -0.086526 |
| MAD | | | 0.102655 | 0.109204 | 0.0551291 | 0.112650 | 0.0928081 |

[1] A. Kramida, Yu. Ralchenko, J. Reader, and and NIST ASD Team, NIST Atomic Spectra Database (ver. 5.6.1), [Online]. Available: https://physics.nist.gov/asd [2019, September 7]. National Institute of Standards and Technology, Gaithersburg, MD. (2018).
